# Supplementary material for: Beat Pilot Tone (BPT): Simultaneous MR Imaging and RF Motion Sensing at Arbitrary Frequencies
Source: arXiv:2306.10236 source file (2024-06-07)
Supplement: Supplementary file 1 [file supp.pdf]

# Beat Pilot Tone Supplementary Information

Suma Anand<sup>1\*</sup> and Michael Lustig<sup>1</sup>

<sup>1\*</sup>Electrical Engineering and Computer Sciences, University of California, Berkeley, 253 Cory Hall, Berkeley, 94720, CA, USA.

\*Corresponding author(s). E-mail(s): [sanand@berkeley.edu](mailto:sanand@berkeley.edu);  
Contributing authors: [mlustig@eecs.berkeley.edu](mailto:mlustig@eecs.berkeley.edu);

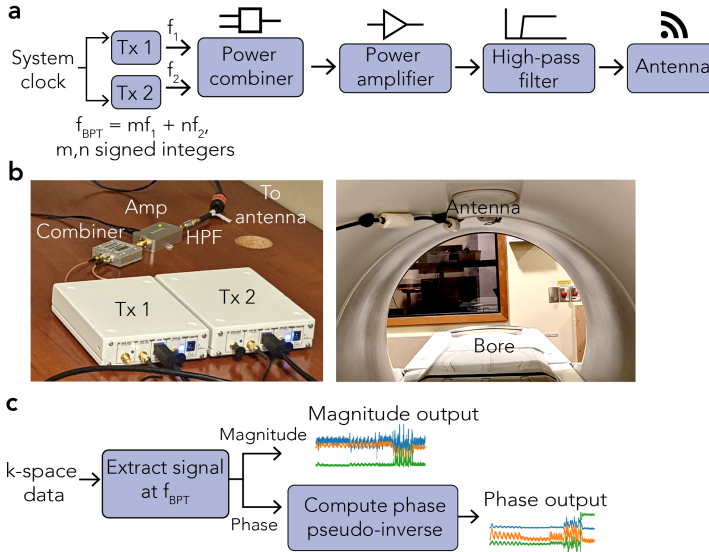

**Supplementary Figure 1** Processing pipeline. a) The acquisition pipeline, in which two tones were generated with two transmitters (e.g., software-defined radios (SDRs)), combined, amplified, high-pass filtered, and transmitted with an antenna. b) Photo of a sample setup, in which the transmitters (left) are USRP B200 SDRs and an antenna (right) is placed at the top of the bore. c) Basic reconstruction pipeline, where the complex signal at  $f_{BPT}$  is extracted from the raw k-space data. The phase is computed by taking the pseudo-inverse of all possible reference coil phases relative to a chosen reference coil.

*BPT*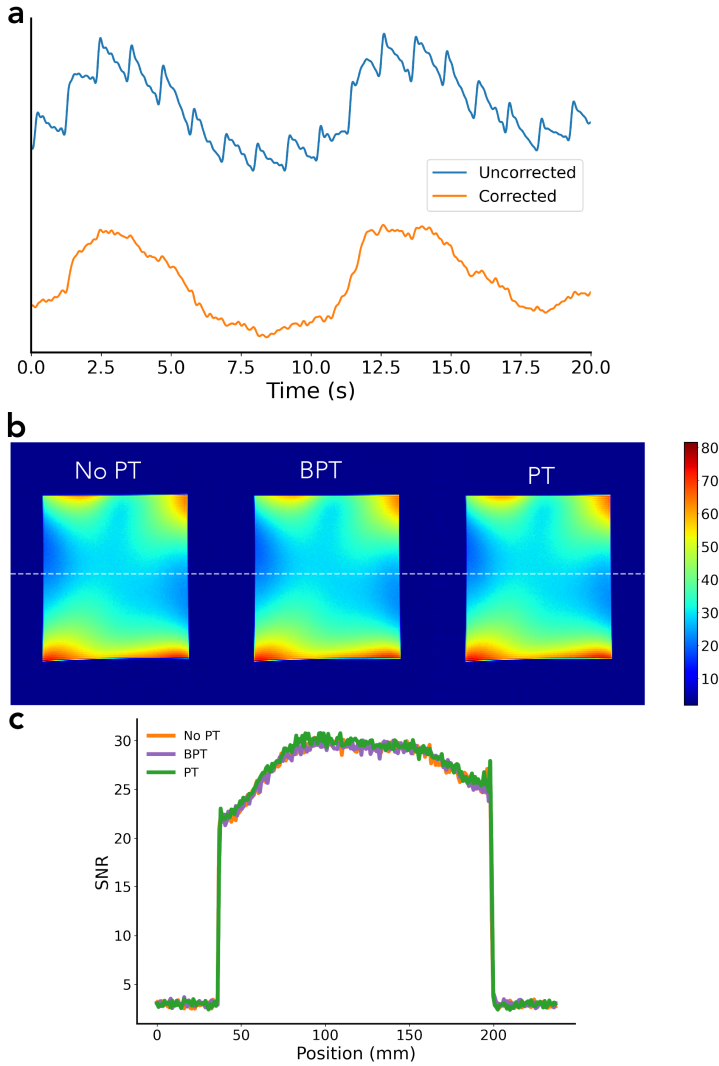

**Supplementary Figure 2** The BPT may be sensitive to certain artifacts. a) If the tx antenna is placed inside the bore, switching gradient fields cause eddy currents to be induced on it, which then vibrate in the scanner due to the Lorentz force from the main magnetic field. For some sequences, this artifact can be approximated from a linear fit and subtracted from the data. An example BPT signal from the head motion experiment is shown here without correction (blue) and with correction using the linear fit approximation (orange). Both signals were low-pass filtered with a cutoff of 5Hz. b) Image SNR was compared in three acquisitions with no PT, BPT, and PT using a uniform phantom with a 32-channel body coil. SNR maps across the three acquisitions are shown. c) Line plots through the center of the maps, indicated by the dashed line.

**Supplementary Table 1** Type and placement of BPT and PT antennas

| Experiment  | BPT Type     | PT Type | BPT Placement        | PT Placement |
|-------------|--------------|---------|----------------------|--------------|
| Rocker      | Log periodic | ”       | Outside              | ”            |
| Respiratory | 4G LTE       | Loop    | Top of bore          | Top of bore  |
| Cardiac     | 4G LTE       | Loop    | Top of bore          | Top of bore  |
| dBCG        | Bluetooth    | Loop    | Top of bore          | On chest     |
| Head        | 2 × 4G LTE   | ”       | Top and side of bore | ”            |

This table shows the type and placement of antennas for BPT and PT. Ditto marks (”) indicate that the antenna or placement was the same, e.g. the same log periodic antenna was used to transmit both BPT and PT.

**Supplementary Table 2** 2.4GHz BPT Hardware

| Hardware element | Model                                    | Company        |
|------------------|------------------------------------------|----------------|
| Transmitter      | USRP B200                                | Ettus Research |
| Power combiner   | ZN2PD-63+                                | Minicircuits   |
| Amplifier        | Sunhans 2.4GHz 34dBm WiFi Signal Booster | Sunhans        |
| High Pass Filter | VHF-440+                                 | Minicircuits   |

The hardware setup for transmitting the BPT at 2.4GHz.

**Supplementary Table 3** Cardiac BPT hardware

| $f_1$ (MHz) | $f_2$ (MHz) | Amplifier                   | High Pass Filter | Antenna |
|-------------|-------------|-----------------------------|------------------|---------|
| 127.8       | N/A         | None                        | None             | Loop    |
| 300         | 427.8       | None                        | VHF-145+         | 4G LTE  |
| 800         | 927.8       | None                        | VHF-440+         | 4G LTE  |
| 1200        | 1327.8      | None                        | VHF-440+         | 4G LTE  |
| 1800        | 1927.8      | None                        | VHF-440+         | 4G LTE  |
| 2400        | 2527.8      | Sunhans WiFi Signal Booster | VHF-440+         | 4G LTE  |

The hardware setup for the cardiac experiment, in which the frequency was swept from 127.8MHz to 2.4GHz in steps of approximately 500MHz. The first column was the PT, so only a single SDR was used without an amplifier or filter.

**Supplementary Table 4** Filtering details

| Experiment  | Figure | Filter cutoff (Hz)                       | Artifact correction |
|-------------|--------|------------------------------------------|---------------------|
| Rocker      | 3      | 5                                        | None                |
| Vibration   | 4      | 1 for < 863.9MHz ; 5 for $\geq$ 863.9MHz | None                |
| Respiratory | 5      | 2                                        | None                |
| Cardiac     | 6      | 3 for < 863.9MHz; 15 for $\geq$ 863.9MHz | None                |
| dBCG        | 7      | 15                                       | None                |
| Head        | 8      | 0.5                                      | Linear fit          |

Filtering and artifact correction details for each experiment, with corresponding Figure number in the second column.
